# Supplementary material for: On self similarity and coarsening rate of a convecting bicontinuous phase separating mixture: effect of the viscosity contrast
Source: arXiv:1709.01299 source file (2018-09-10)
Supplement: Supplementary file 1 [file suplemental.pdf]

# Details of the numerical implementation and of the method of analysis

Hervé Henry[1] and György Tegze[2]
[1] *Laboratoire de Physique de la Matière Condensée, École Polytechnique, CNRS, Université Paris-Saclay, 91128 Palaiseau Cedex, France* and
[2] *Wigner Research Centre for Physics, P.O. Box 49, H-1525 Budapest, Hungary*

Here, to help the reproducibility of our results, here we present in more details the model we used for our simulations, and we describe the numerical implementation and describe how simulation data were analyzed, that is how quantities such as the curvatures were computed and how PDFs of the curvatures were estimated. In addition we present curves obtained with different parameter values that confirm the genericity of our results.

## I. DETAILS OF THE MODEL

We assume, that the Helmholtz free energy of an inhomogeneous two-component system can be expressed as a functional of the concentration. In the simplest case, the free energy has the well known, symmetric Cahn-Hilliard form [1]:

$$\mathcal{F} = \int \epsilon^2 (\nabla c)^2 + A \times (c^2 (c-1)^2) \tag{1}$$

,

herein our choice of the parameters were $A = 0.0625 \times 4$ and $\epsilon_c^2 = 0.04 \times 4$, that corresponds to the values used by Kendon et al. in the run 29 of [2]. Also we have used Kendon's results as reference when validating our implementation of the model. In a two-phase equilibrium, can be realized by minimizing the free-energy functional the phase boundary is characterized by a diffuse interface, where the composition vary between $c = 0$ and $c = 1$ as a hyperbolic tangent function: $(1 + \tanh(x/w_{int}))/2)$. The diffuseness of the phase boundary is characterized by the interface width $w_int$, and it is relates to the parameters of the free energy as $w_{int} = \sqrt{4\varepsilon_c^2/A} = 1.6$. The free energy also defines the equilibrium surface tension for our choice of parameters as $\gamma = 0.042$. We mention here, that the relevant parameter in our numerical experiments is the surface tension, since the interface thickness plays minor in the coarsening regime, where the characteristic length of the microstructure is considerably larger, that the interface width.

While the derivation of the diffusion fluxes from the free-energy functional is widely known, various formalisms that represent a reversible capillary stresses often leads to confusion. Formally, reversible stress $\mathbb{R}$ relates to the free-energy as $\nabla \cdot \mathbb{R} = -c\nabla(\delta\mathcal{F}/\delta c)$ through the least action principle for conserved variables. Accordingly the reversible stress tensor can be written in the following form [3]:

$$\frac{\mathbb{R}}{\rho} = \mathbb{I}\left[\phi - c\frac{\partial\phi}{\partial c} + \epsilon\left\{\frac{1}{2}(\nabla c)^2 + c\nabla^2 c\right\}\right] - \epsilon\,(\nabla c \otimes \nabla c) \tag{2}$$

where $\phi = Ac^2(1-c)^2$ is the local contribution to the free-energy, and the corresponding terms in $\mathbb{R}$ represents osmotic pressure. The diagonal elements of first term in the RHS are isotropic therefore represents a pressure $p$ and therefore eq.2 can be, in the case of incompressible fluids, rewritten:

$$\frac{\mathbb{R}}{\rho} = -p - \epsilon\,(\nabla c \otimes \nabla c) \tag{3}$$

We note here, that $p$ may also include additional Lagrangian multipliers that relate to the divergence free projection, or guarantee $\sum c_i = 1$ in a multicomponent system [4]. In our incompressible case the pressure term does not contribute to the fluid flow. As a result the second term of $\mathbb{R}$ is solely responsible for capillary stress.

## II. NUMERICAL IMPLEMENTATION

Pseudo-spectral methods has long been used to compute turbulent flows [5, 6], and multi-phase flows [7] due to their high spatial accuracy(i.e. both amplitude and phase errors decaying exponentially with the resolution). The low dispersion characteristics of the method ensures, that the subtle balance between inertial and viscous forces will not be modified by the numerical dissipation. A further advantage of the method, that a numerically more stable solution is

possible using the operator splitting technique at no extra cost: using backward Euler time integration for the viscous term, while forward Euler for the remaining terms. Besides is is straightforward to "force" incompressibility using the Helmholtz theorem: projection to divergence-free velosity field does not require to explicitly compute pressure, that used to force incompressibility.

While the spectral discretization is straightforward for most of the terms in the equations, the effective computing of spatially varying viscous dissipation needs special treatment: again the operator splitting technique is applied, following Zhu et al. the viscosity term is split to a homogeneous and an inhomogeneous term that ensures improved stability [8]. Our implementation of the method is featuring concurrent execution using the MPI standard. The measured scaling of efficiency on massively parallel hardware (IBM Blue Gene/Q) is excellent which allowed us to run simulations of domain of size $512^3$ and $1024^3$. The later grid size was used to confirm result obtained using the smaller grid and to have a statistically representative sample when computing the PDFs of the curvatures. The code was validated by comparing our simulations results with the Run 28 of [2] and using the same quantity to measure a characteristic length. The coarsening rate we computed matched the one from [2] with a relative error smaller than 2% which is excellent considering that our incompressible fluid flow model differs from Lattice Boltzmann Model, that has been used in the reference work. Besides comparing to a reference solution, we have performed convergence analysis via varying the grid-spacing between $\delta x = 1$ and $\delta x = 4$. It was concluded, that reasonable accuracy can be obtained up to $\delta x = 2$. We note, that in practice, the spatial resolution is limited by the computations of the principal curvatures. Similarly, the convergence on $\delta t$ is investigated, and the reasonable time resolution was dependent on the characteristic flow velocity.

The initial condition, in order to save some computing time and to avoid that the flow affects the early stage of phase separation in an uncontrolled manner was obtained by filling the computational domain with small spheres (of radius $\approx 2$) of one phase until the desired volume fraction was reached. In the case where the volume fraction is 0.5, using oblate or prolate ellipsoids with an aspect ration up to 10 did not change the statistics of the self-similar steady state.

## III. DETAILS OF THE METHOD OF ANALYSIS

It is common that the coarsening rate is described by the varying characteristic length of the interconnected domains. It can be either the ratio of the $n^{th}$ and $(n+1)^{th}$ moment of the structure function where $n$ can be chosen arbitrarily or it can be the ratio of a characteristic volume over a characteristic surface: $l = V/S$. To evaluate the latter can be challenging, when using diffuse interface models where the interface is defined implicitly, since resolving even the smallest features of the topology is required. As an alternative, we take advantage of the fact that here, the total surface energy in the computation domain can be measured with high accuracy. Then dividing it by the surface tension of the planar interface approximates accurately the characteristic surface.

$$S = \int \epsilon^2 (\nabla c)^2 + A \times (c^2(c-1)^2)/\gamma. \tag{4}$$

Besides the length-scale, the curvature of the interfaces is characteristic to the microstructure. Computing it with accuracy is a challenging task. In a similar fashion to[9], to avoid discretization effects, when extracting the curvature data, we first interpolated $c$ on a finer grid with grid spacing $\Delta x = 0.5$, ran a few CH steps (without flow) in order to regularize the interface without changing the topology and finally used implicit formulas for the curvature[10] :

$$\kappa_g = \frac{\nabla c H^* \nabla c}{(\nabla c)^4} \tag{5}$$

$$\kappa_m = \frac{\nabla c H \nabla c - (\nabla c)^2 \mathrm{trace}(H)}{2|\nabla c|^3} \tag{6}$$

where $H$ is the symmetric Hessian matrix: $H_{ij} = \partial^2_{x_i,x_j} c$ and $H^*$ is the co-matrix of $H$. The principal curvatures can easily be computed:

$$\kappa_{1,2} = \kappa_m \pm \sqrt{\kappa_m^2 - \kappa_g} \tag{7}$$

Once the curvature field were computed, the contribution of each point to the Probability Distribution Functions (PDFs) of the curvature was taken to be the local surface energy density $e$. Such an approach has the advantage of avoiding the computation of the explicit interface and then interpolating the curvature on the interface. It suffers from the fact that the curvature are not computed at the exact interface and therefore some limited interface thickness (vanishing with $w_{int}/l$) effects are expected.

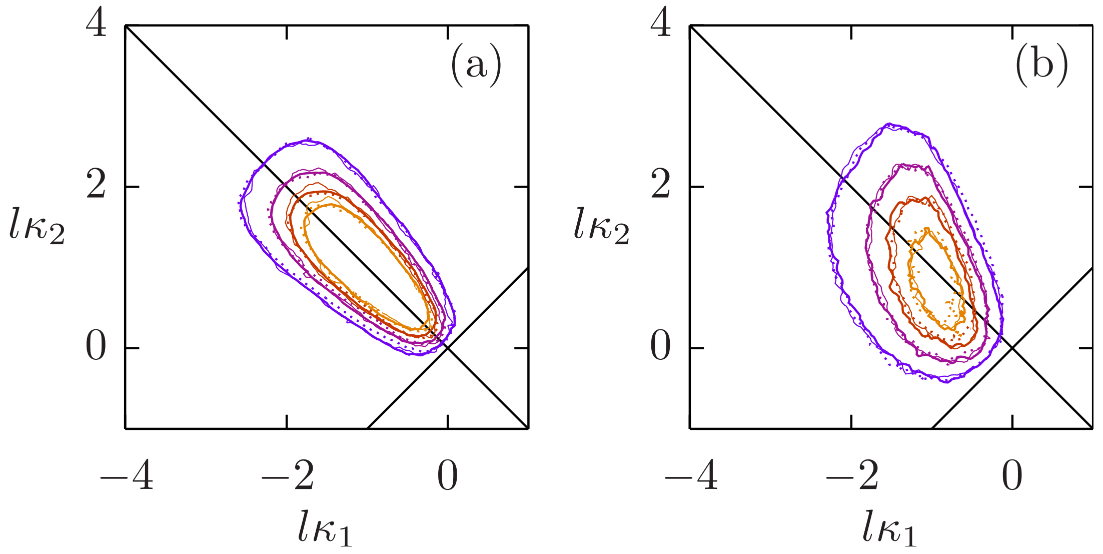


FIG. 1. PDFs of the curvatures for different test case that are the same as the ne presented in the main text. The thick dashed and solid lines correspond to $\nu_{eff} = 4$ and $\nu_{eff} = 16$ while the thin solid line corresponds to $\nu_{eff} = 8$. In (a) the viscosity contrast is 1 and in (b) it is 128.

The genius is a topological invariant of the structure (related to the Euler's characteristic) and is

$$g = (1 - \frac{1}{4\pi}\int \kappa_g). \tag{8}$$

It characterizes the topology of the surface and depends on the number of cavities, holes and inclusions of the microstructure. In a self-similar growth one expects the density of such topological structure to scale as $l^{-3}$. As a result the rescaled genius is simply $g/(V/l^3)$ should be constant in and it indicates the complexity of the topology of the microstructure. In the peculiar case of our diffuse interface model we used the following formula for the genius:

$$g = (1 - \frac{1}{4\pi}\int e\kappa_g/\gamma) \tag{9}$$

where $e$ is the local surface energy density.

## IV. COMPLEMENTARY RESULTS

The results presented in the main text are only a part of the simulations we performed during this work. Here, in order to show that the behaviour is actually robust to parameter changes, we present the results of simulations performed with different parameter sets and different initial conditions. In addition, since such plots are commonly used in the literature, we also plot the structure functions corresponding to our simulations and give a rationale for not limiting ourselves to them.

First, we have checked, as one would expect, that the microstructure characteristics are independent of the viscosity, but solely depends on the viscosity contrast. To this purpose we present in fig.1 the PDFs of the main curvatures for simulations performed with $\nu_{eff} = 4,\ 8,$ and 16 and for two values of the viscosity contrast $VC = 1$ and 128. One can see on the figure that the contour lines of the PDFs (using a linear scale) are very close to each other for each of the values of $\nu_{eff}$. Moreover, we have checked that in all cases the self similar behaviour holds. This clearly indicates that the self similar final microstructure is independent of the viscosity as long as inertial effects are not present.

In a second step, we have performed simulations using different initial conditions in order to check that it does not have influence on the characteristics of the self similar microstructure. To this purpose we performed simulations with a given value of the viscosity contrast $VC = 128$ until the self similar regime was reached (i.e. a regime where the rescaled PDF of curvatures is stationary). Then the viscosity contrast was modified (either to $VC = 1$ or $VC = 1/128$ by inverting the phases). In both cases after a short transient regime, the PDF of the curvatures was the same as the one observed in simulations with a constant value of $VC$. This indicates that the characteristics of the pattern are independent of the initial condition.

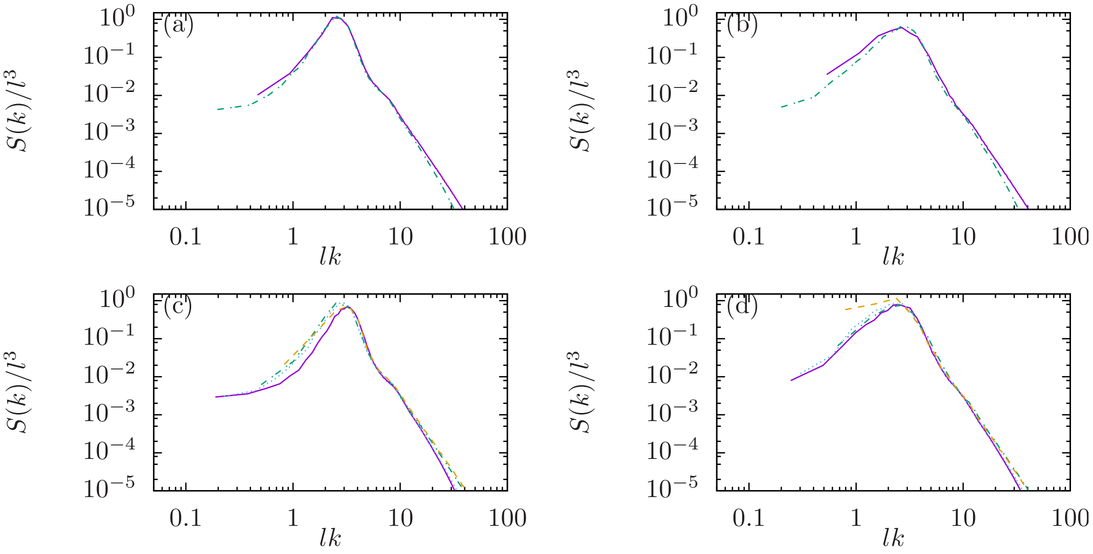


FIG. 2. Structure function for VC=1 (a) and VC=128(b) obtained at two times corresponding to $l \approx 30$ and $l \approx 80$. during our simulations after rescaling. They indicate also self-similarity. It is worth mentionning that here the shoulder present in (a) is vanishing in (b). This was attributed to inertial effects in a prefectly symmetric case. Here it is not the case. In (c) (resp. (d)) we present for VC=1 (resp. 128) a superimposition of the curves for $\sqrt{\nu_h \nu_l} = 4$ and $\sqrt{\nu_h \nu_l} = 16$, (the reynolds number being kept constant thanks to a proper change in the fluid density and characteristic lengths are similar to the one in (a) and (b)) indicating that the effect of viscosity is neglectable on the pattern itself.

These results show that the phenomenon described in the main text are robust (in the limits of viscous coarsening) to parameter changes and to initial condition changes.

Now, for the sake of comparison with other works we present briefly the structure functions in the cases $VC = 1$ and $VC = 128$. They are represented in fig. 2 With no surprise, they confirm the self-similar nature of the structure since after rescaling by the characteristic length, the curves obtained for a given value of $VC$ collapse very well on a single master curve. The comparison of our $VC = 1$ curve and the $VC = 1$ curve presented in [2] shows a very good qualitative agreement. When comparing the $VC = 128$ curve with the $VC = 1$ curve, one can see that the $VC = 128$ curve has a broader maximum than the $VC = 1$ curve hand does not present a marked shoulder at moderatedly high $kl$. This indicates that a broader distribution of length scales is present in the microstructure and it can also be seen when considering the PDFs of the curvatures since there, the maximum of the distribution is less marked in the case $VC = 128$ than in the case $VC = 1$. But, the structure function cannot capture the symmetry breaking induced by the viscosity contrast between the phases that is clear when considering the PDFs of $\kappa_{1,2}$ where the contour lines are no longer symmetric with respect to the axis $\kappa_1 = -\kappa_2$.


[1] J. W. Cahn and J. E. Hilliard, The Journal of Chemical Physics **28**, 258 (1958).
[2] V. M. Kendon, M. E. Cates, I. Pagonabarraga, J.-C. Desplat, and P. Blandon, Journal of Fluid Mechanics **440**, 147 (2001).
[3] B. Z. Shang, N. K. Voulgarakis, and J.-W. Chu, The Journal of Chemical Physics **135**, 044111 (2011), http://dx.doi.org/10.1063/1.3615719.
[4] G. I. Tóth, M. Zarifi, and B. Kvamme, Phys. Rev. E **93**, 013126 (2016).
[5] S. A. Orszag, Physics of Fluids **12**, II (1969).
[6] S. A. Orszag and G. S. Patterson, Phys. Rev. Lett. **28**, 76 (1972).
[7] C. Liu and J. Shen, Physica D: Nonlinear Phenomena **179**, 211 (2003).
[8] J. Zhu, L.-Q. Chen, J. Shen, and V. Tikare, Phys. Rev. E **60**, 3564 (1999).
[9] Y. Kwon, K. Thornton, and P. W. Voorhees, EPL (Europhysics Letters) **86**, 46005 (2009).
[10] R. Goldman, Computer Aided Geometric Design **22**, 632 (2005).
